# Supplementary material for: Beyond socket options: making the Linux TCP stack truly extensible
Source: arXiv:1901.01863 source file (2019-05-22)
Supplement: Supplementary file 1 [file appendix.tex]

\section*{Appendix: BPF programs example}

\begin{lstlisting}[language=C, caption=BPF program to write IW option]
struct tcp_option {
	__u8 kind;
	__u8 len;
	__u16 data;
}
SEC("sockops")
int bpf_insert_option(struct bpf_sock_ops *skops) {
	struct tcp_option opt = {
		.kind = 66,     // option kind number
		.len = 4,       // of this option struct
		.data = 20,	    // # MSS
	};
	int rv = 0;
	int option_buffer;
	
	// for simplicity, we excluded the peer IP check
	switch (skops->op) {
	case BPF_SOCK_OPS_ACTIVE_ESTABLISHED_CB:
		// activate option writing flag
		rv = bpf_sock_ops_cb_flags_set(skops,
					BPF_SOCK_OPS_OPTION_WRITE_FLAG);
		break;
	case BPF_TCP_OPTIONS_SIZE_CALC:
		// adjust total option len, not over 40 Bytes
		int option_len = sizeof(opt);
		int total_len = skops->args[1];
		if (total_len + option_len <= 40)
			rv = option_len;
		break;
	case BPF_TCP_OPTIONS_WRITE:
		// put struct option into reply field
		memcpy(&option_buffer, &opt, sizeof(int));
		rv = option_buffer;
		// will not insert option after 1st data packet
		if (skops->data_segs_in > 1)
			bpf_sock_ops_cb_flags_set(skops, 0);
		break;
	default:
		rv = -1;
	}
	skops->reply = rv;
	return 1;
}
\end{lstlisting}
